# Supplementary material for: Flow Score Distillation for Diverse Text-to-3D Generation
Source: arXiv:2405.10988 source file (2024-07-28)
Supplement: Supplementary file 1 [file appendix.tex]

% \documentclass[runningheads]{llncs}

% % ---------------------------------------------------------------
% % Include basic ECCV package
 
% % TODO REVIEW: Insert your submission number below by replacing '*****'
% % TODO FINAL: Comment out the following line for the camera-ready version
% \usepackage[review,year=2024,ID=2501]{eccv}
% % TODO FINAL: Un-comment the following line for the camera-ready version
% %\usepackage{eccv}

% % OPTIONAL: Un-comment the following line for a version which is easier to read
% % on small portrait-orientation screens (e.g., mobile phones, or beside other windows)
% %\usepackage[mobile]{eccv}


% % ---------------------------------------------------------------
% % Other packages

% % Commonly used abbreviations (\eg, \ie, \etc, \cf, \etal, etc.)
% \usepackage{eccvabbrv}

% % Include other packages here, before hyperref.
% \usepackage{graphicx}
% \usepackage{booktabs}
% \usepackage{algorithm,algorithmic}

% % The "axessiblity" package can be found at: https://ctan.org/pkg/axessibility?lang=en
% \usepackage[accsupp]{axessibility}  % Improves PDF readability for those with disabilities.


% % ---------------------------------------------------------------
% % Hyperref package

% % It is strongly recommended to use hyperref, especially for the review version.
% % Please disable hyperref *only* if you encounter grave issues.
% % hyperref with option pagebackref eases the reviewers' job, but should be disabled for the final version.
% %
% % If you comment hyperref and then uncomment it, you should delete
% % main.aux before re-running LaTeX.
% % (Or just hit 'q' on the first LaTeX run, let it finish, and you
% %  should be clear).

% % TODO FINAL: Comment out the following line for the camera-ready version
% \usepackage[pagebackref,breaklinks,colorlinks,citecolor=eccvblue]{hyperref}
% % TODO FINAL: Un-comment the following line for the camera-ready version
% %\usepackage{hyperref}

% % Support for ORCID icon
% \usepackage{orcidlink}


% \newcommand{\bd}{\boldsymbol}
% \newcommand{\E}{\mathbb{E}}
% \newcommand{\dd}{\mathrm{d}}
% \newcommand{\Normal}{\mathcal{N}(\bd{0},\bd{I})}
% \newcommand{\Lsds}{L_{\text{SDS}}^\theta}
% \newcommand{\Lfsd}{L_{\text{FSD}}^\theta}
% \newcommand{\lsds}{L_{\text{sds}}^\theta}
% \newcommand{\lsdsdd}{L_{\text{sds-2d}}^\theta}
% \newcommand{\gc}{\bd{g}_\theta(\bd{c})}
% \newcommand{\ec}{\bd{\epsilon}(\bd{c})}
% \newcommand{\xo}{\hat{\bd{x}}^{\text{c}}_t}
% \newcommand{\xc}{\hat{\bd{x}}^{\text{gt}}_t}
% \newcommand{\epsf}{\tilde{\bd{\epsilon}}}
% \newcommand{\window}{\bd{W}_{(W\frac{\phi_{\text{cam}}}{2\pi},H\frac{\theta_{\text{cam}}}{\pi})}}

% \begin{document}

% % ---------------------------------------------------------------
% % TODO REVIEW: Replace with your title
% \appendix
% \title{Appendix}
% \maketitle

% \section{Quantitative Results}
% We compute several metrics for 3D generation results with SDS\cite{poole2022dreamfusion, wang2023score} and FSD. The hyperparameters are kept the same as those in \cref{app-sec:additional}. When using Stable Diffusion\cite{song2020denoising} as backbone, we use 16 prompts and 4 random seeds for each prompt (\cref{app-tab:sd}). When using MVDream\cite{shi2023mvdream} as backbone, we also use 16 prompts and 4 random seeds for each prompt (\cref{app-tab:mvdream}).
% \begin{table}[htb]
%   \caption{Stable Diffusion\cite{song2020denoising} as backbone
%   }
%   \label{app-tab:sd}
%   \centering
%   \begin{tabular}{@{}c|ccc@{}}
%     \toprule
%     Method & CLIP ($\uparrow$) & IS ($\uparrow$) & CROSS-FID ($\uparrow$)\\
%     \midrule
%     DDIM Images 
%     & $33.72\pm1.83$ & $1.68\pm0.55$ & -\\
%     \midrule
%     SDS\cite{poole2022dreamfusion,wang2023score} 
%     & $32.57\pm1.43$ & $1.58\pm0.47$ & $106.5\pm58.3$\\
%     FSD(ours) 
%     & $\mathbf{32.72\pm1.56}$ & $\mathbf{1.78\pm0.49}$ & $\mathbf{141.8\pm57.9}$\\
%   \bottomrule
%   \end{tabular}
% \end{table}

% \begin{table}[htb]
%   \caption{MVDream\cite{shi2023mvdream} as backbone}
%   \label{app-tab:mvdream}
%   \centering
%   \begin{tabular}{@{}c|ccc@{}}
%     \toprule
%     Method & CLIP ($\uparrow$) & IS ($\uparrow$) & CROSS-FID ($\uparrow$)\\
%     \midrule
%     DDIM Images & 
%     $34.64\pm2.56$ & $2.02\pm0.47$ & -\\
%     \midrule
%     SDS\cite{poole2022dreamfusion,wang2023score} & 
%     $\mathbf{30.93\pm3.40}$ & $1.77\pm0.37$ & $86.6\pm33.4$\\
%     FSD(ours) & 
%     $30.12\pm3.07$ & $\mathbf{2.13\pm0.35}$ & $\mathbf{174.8\pm44.5}$\\
%   \bottomrule
%   \end{tabular}
% \end{table}

% \subsubsection{CLIP score}
% We compute CLIP score\cite{hessel2021clipscore, radford2021learning} using ViT-B/32 to measure the semantic similarity between the renderings of the generated 3D object and the input text prompt. We sample 24 views for each prompt and each seed when computing CLIP score. 

% \subsubsection{IS score}
% We compute IS score\cite{salimans2016improved} to measure both the image quality and diversity. We first compute the IS scores of sampled views for each prompt and then average the IS scores across prompts.

% \subsubsection{CROSS-FID score}
% To directly measure the diversity of generation results, it is natural to measure the inception distance between different generated samples. We first sample 24 views for each prompt and each seed. Then we separate the images corresponding to random seeds 0, 1 and 2, 3 into two sets of images. We compute FID\cite{heusel2017gans} of the two sets of images and average the FID score across prompts. We term this score as CROSS-FID score since it is different from the standard way of using FID to evaluate GANs\cite{heusel2017gans}.

% % TODO user study?

% \section{Additional Experiment Results}
% \label{app-sec:additional}
% \subsection{Additional Generation Results}
% \begin{figure}[tp]
%   \centering
% \includegraphics[width=\linewidth]{assets/compare.pdf}
%   \caption{\textbf{Comparisons between FSD and SDS-like baseline methods.} We present results of FSD and compare them to baseline methods, namely ProlificDreamer (VSD)\cite{wang2024prolificdreamer}, SDS\cite{poole2022dreamfusion, wang2023score}, CSD\cite{ho2022classifier}. We use random seeds from 0 to 3 for each prompt.
%   }
%   \label{app-fig:baselines}
% \end{figure}
% \begin{figure}[tp]
%   \centering
% \includegraphics[width=\linewidth]{assets/app-sd.pdf}
%   \caption{\textbf{Experiment results of FSD and SDS\cite{poole2022dreamfusion, song2020score} with Stable Diffusion\cite{song2020denoising} as backbone.}
%   }
%   \label{app-fig:sd}
% \end{figure}
% \begin{figure}[tp]
%   \centering
% \includegraphics[width=\linewidth]{assets/app-mvdream-1.pdf}
%   \caption{\textbf{Experiment results of FSD and SDS\cite{poole2022dreamfusion, song2020score} with MVDream\cite{shi2023mvdream} as backbone.}
%   }
%   \label{app-fig:mvdream}
% \end{figure}
% We provide additional 3D experiment results using FSD and other SDS-like methods in \cref{app-fig:baselines}, \cref{app-fig:sd} and \cref{app-fig:mvdream}.

% Specifically, in \cref{app-fig:baselines}, we present results of FSD and compare them to baseline methods, namely ProlificDreamer (VSD)\cite{wang2024prolificdreamer}, SDS\cite{poole2022dreamfusion, wang2023score}, CSD\cite{ho2022classifier}. In \cref{app-fig:sd}, we provide additional comparisons between SDS and FSD with Stable Diffusion\cite{song2020denoising} as the backbone Diffusion Model. In \cref{app-fig:mvdream}, we provide additional comparisons between SDS and FSD with MVDream\cite{shi2023mvdream} as the backbone Diffusion Model. We do not provide experiment results with Diffusion Models designed for novel view synthesis (\eg SyncDreamer\cite{liu2023syncdreamer}) since we found FSD does not improve the diversity of the back view of an object significantly given the front view when using Diffusion Models of such category.
% % TODO sds/fsd/vsd/csd/ism?

% \subsection{Additional Ablations}

% \begin{figure}[t]
%   \centering
%   \begin{subfigure}{0.18\linewidth}
%     \includegraphics[width=\linewidth]{assets/mvdream-theta/120.png}
%     \caption*{$\Theta=120^{\circ}$}
%   \end{subfigure}
%   \hfill
%   \begin{subfigure}{0.18\linewidth}
%     \includegraphics[width=\linewidth]{assets/mvdream-theta/180.png}
%     \caption*{$\Theta=180^{\circ}$}
%   \end{subfigure}
%   \hfill
%   \begin{subfigure}{0.18\linewidth}
%     \includegraphics[width=\linewidth]{assets/mvdream-theta/240.png}
%     \caption*{$\Theta=240^{\circ}$}
%   \end{subfigure}
%   \hfill
%   \begin{subfigure}{0.18\linewidth}
%     \includegraphics[width=\linewidth]{assets/mvdream-theta/300.png}
%     \caption*{$\Theta=300^{\circ}$}
%   \end{subfigure}
%   \hfill
%   \begin{subfigure}{0.18\linewidth}
%     \includegraphics[width=\linewidth]{assets/mvdream-theta/360.png}
%     \caption*{$\Theta=360^{\circ}$}
%   \end{subfigure}
%   \caption{\textbf{Ablation on other hyperparameters in $\ec$.} We use a parameter $\Theta$ to control the size of noise world map ($H$ and $W$) in $\ec$. When $\Theta$ is larger, the ``radius $r_+$'' (\cref{app-eq:rp-theta} and \cref{app-eq:rp-phi}) of the noise world map is smaller and FSD trends to generate smaller 3D models. In practice, we found FSD is prone to the parameter $\Theta$.
%   }
%   \label{app-fig:thetas}
% \end{figure}

% We use a parameter $\Theta$ to control the noise world-map's size ($H$ and $W$). $H$ and $W$ are determined by $\Theta$ according to $H=H_{\text{hidden}}\frac{\pi}{\Theta}$ and $W=W_{\text{hidden}}\frac{2\pi}{\Theta}$. We visualize the results corresponding to different $\Theta$s in \cref{app-fig:thetas}.


% \begin{figure}[t]
%   \centering
%   \hfill
%   \begin{subfigure}{0.45\linewidth}
%       \includegraphics[width=\linewidth]{assets/vanilla/0.png}\\
%       \includegraphics[width=\linewidth]{assets/vanilla/1.png}\\
%       \includegraphics[width=\linewidth]{assets/vanilla/2.png}\\
%       \includegraphics[width=\linewidth]{assets/vanilla/3.png}
%       \caption{vanilla constant noise function}
%   \end{subfigure}
%   \hfill
%   \begin{subfigure}{0.45\linewidth}
%       \includegraphics[width=\linewidth]{assets/world-map/0.png}\\
%       \includegraphics[width=\linewidth]{assets/world-map/1.png}\\
%       \includegraphics[width=\linewidth]{assets/world-map/2.png}\\
%       \includegraphics[width=\linewidth]{assets/world-map/3.png}
%       \caption{world-map noise function (proposed)}
%   \end{subfigure}
%   \hfill
%   \caption{\textbf{Ablation on design of $\ec$.} We use noise function $\ec$ to align noise prior in FSD. We present RGB maps and depth maps of the generated samples using random seeds from 0 to 3. A vanilla constant function may result in holes on the surfaces. In contrast, the world-map noise function will not lead to any obvious flaws.
%   }
%   \label{app-fig:vanilla}
% \end{figure}

% We also provide an additional comparison between the vanilla constant noise function and the world-map noise function in \cref{app-fig:vanilla}. We find the constant noise function may harm the geometry of the generation results.

% \subsection{Additional Experiments on Noise Prior}

% \begin{figure}[tbh]
% \centering
% \includegraphics[width=0.95\linewidth]{assets/edit-app.pdf}
%   \caption{\textbf{Impact of initial noise $\epsf$.} We provide additional 2D experiment results generated by FSD show the impact of the initial noise $\epsf$. The patches framed with the same color in the same row share the same initial noise patches. 
%   }
%   \label{app-fig:fsd-2d-local}
% \end{figure}
% We provided additional generation results of FSD on 2D image space with shuffled or flipped initial noise in \cref{app-fig:fsd-2d-local}. The patches framed with the same color in the same row share the same initial noise patches $\epsf$.


% \section{Implementation Details}
% \subsection{3D Experiments using FSD}

% The backbone Diffusion Model for Fig. 1 in the main text is MVDream\cite{shi2023mvdream}. The configuration for this figure is the same as Fig. 7 in the main text.

% We use sqrt-annealing proposed by HiFA\cite{zhu2023hifa} for 3D experiments in this work. We use the same CFG\cite{ho2022classifier} scale for SDS\cite{shi2023mvdream, wang2023score} and FSD. We use CFG=1 when applying image loss trick\cite{zhu2023hifa} since we find the reconstructed images are unrealistic when the CFG scale is large, which is not good guidance. We follow the default setting of threestudio\cite{threestudio2023} code base for other hyperparameters. We keep the iteration number and learning rate of FSD the same as SDS\cite{shi2023mvdream, wang2023score} in 3D experiments. We mainly conduct our experiments using NeRF representation\cite{muller2022instant} since SDS-like methods are not sensitive to the form of 3D representations.

% \subsection{2D Experiments using FSD}

% \begin{table}[tb]
%   \caption{Implementation details on 2D experiments with FSD.}
%   \label{app-tab:impl-2d}
%   \centering
%   \begin{tabular}{@{}l|cccccc@{}}
%     \toprule
%     Methods Name & SDS\cite{poole2022dreamfusion,wang2023score} & NFSD\cite{katzir2023noise} & VSD\cite{wang2024prolificdreamer} & FSD(ours) & DDIM\cite{song2020denoising}\\
%     \midrule
%     Iteration Num & 500 & 500 & 500 & 500 & 50\\
%     CFG\cite{ho2022classifier} & 100 & 7.5 & 7.5 & 7.5 & 7.5\\
%     Learning Rate & 2e-2 & 2e-2 & 2e-2 & 3e-3 & -\\
%     Optimizer & Adam\cite{kingma2014adam} & Adam & Adam & Adam & -\\
%     Timestep Annealing & linear & linear& linear& linear& -\\
%   \bottomrule
%   \end{tabular}
% \end{table}
% Here we describe the details of the experiments on 2D images with FSD in the main text. For Fig. 3 in the main text, we show the implementation details in \cref{app-tab:impl-2d}. Below, we provide the loss functions for convenient reference.

% Let denote the prediction of Diffusion Models as $\bd{\epsilon}_y^t=\bd{\epsilon}_\phi(\bd{x}_t|y,t)$ and $c$ the classifier-free-guidance (CFG)\cite{ho2022classifier} scale. Then
% \begin{equation}
%     \nabla_\theta L_{\text{SDS}}^\theta = \E_{\bd{\epsilon},\bd{c},t}  \left[  \left(c \cdot (\bd{\epsilon}^t_y-\bd{\epsilon}^t_\emptyset)+(\bd{\epsilon}^t_\emptyset-\bd{\epsilon})\right)\frac{\partial \gc}{\partial \theta}\right]
% \end{equation}
% is the loss function of SDS\cite{poole2022dreamfusion, wang2023score}, where $\emptyset$ is the empty prompt.

% \begin{equation}
%     \nabla_\theta L_{\text{NFSD}}^\theta = \E_{\bd{\epsilon},\bd{c},t}  \left[  \left(c \cdot (\bd{\epsilon}^t_y-\bd{\epsilon}^t_\emptyset)+(\bd{\epsilon}^t_\emptyset-\bd{\epsilon}^t_{y_{\text{neg}}})\right)\frac{\partial \gc}{\partial \theta}\right]
% \end{equation}
% is the loss function of NFSD\cite{katzir2023noise}, where $y_{\text{neg}}$ is a text negative prompt.

% \begin{equation}
%     \nabla_\theta L_{\text{VSD}}^\theta = \E_{\bd{\epsilon},\bd{c},t}  \left[  \left(c \cdot (\bd{\epsilon}^t_y-\bd{\epsilon}^t_\emptyset)+(\bd{\epsilon}^t_\emptyset-\bd{\epsilon}^t_{\text{lora}})\right)\frac{\partial \gc}{\partial \theta}\right]
% \end{equation}
% is the loss function of VSD\cite{wang2024prolificdreamer}, where $\bd{\epsilon}^t_{\text{lora}}$ the Diffusion Model fine-tuned by LoRA\cite{hu2021lora}. 

% \begin{equation}
%     \nabla_\theta L_{\text{FSD}}^\theta = \E_{\bd{c},t}  \left[  \left(c \cdot (\bd{\epsilon}^t_y-\bd{\epsilon}^t_\emptyset)+(\bd{\epsilon}^t_\emptyset-\bd{\epsilon}(\bd{c}))\right)\frac{\partial \gc}{\partial \theta}\right]
% \end{equation}
% is the loss function of FSD. Additionally, $\bd{x}_t = \alpha_t \gc + \sigma_t \ec$ for FSD.

% Our re-implementation of $L_{NFSD}$ is slightly different from the original\cite{katzir2023noise} design of NFSD by ignoring the condition when $t<200$, to keep the formulation simple. In this way, we find $\bd{\epsilon}^t_{\text{lora}}$ used in VSD\cite{wang2024prolificdreamer} may work in a similar way as $\bd{\epsilon}^t_{y_{\text{neg}}}$ in NFSD\cite{katzir2023noise}. As a result, single-particle VSD may not be able to generate diverse samples since it is still mode-seeking, aligning with the observation of ESD\cite{wang2023taming}. But we do not conduct further investigations which are out of the scope of our work.

% \section{Theory of Flow Score Distillation}
% We will provide some additional preliminaries and proof of Proposition 1 in the main text in this section.
% \subsection{Diffusion PF-ODE}
% The Diffusion PF-ODE \cite{song2020score} can be written in the following form:
% \begin{equation}
%   \frac{\dd \bd{x}_t}{\dd t} = f(t) \bd{x}_t - \frac{1}{2}g^2(t) \nabla_{\bd{x}} \log p_t(\bd{x}_t|y),\quad
%   \bd{x}_T \sim p_T(\bd{x}_T),\label{eq:pf-ode}
% \end{equation}
% where $f(t) = \frac{\dd \log \alpha_t}{\dd t},\;
% g^2(t) = \frac{\dd \sigma_t^2}{\dd t} - 2 \frac{\dd \log \alpha_t}{\dd t} \sigma^2_t
% $, according to DPM-solver\cite{lu2022dpm}. To get Eq. (5) in the main text, we take the derivative of $\bd{x}_t/\alpha_t$:
% \begin{equation}
% \begin{aligned}
%   \frac{\dd (\bd{x}_t/\alpha_t)}{\dd t}
%   =& \frac{1}{\alpha_t}\frac{\dd \bd{x}_t}{\dd t} - \frac{\bd{x}_t}{\alpha_t^2}\frac{\dd \alpha_t}{\dd t}\\
%   =& \frac{1}{\alpha_t}\frac{\dd \bd{x}_t}{\dd t} - \frac{\bd{x}_t}{\alpha_t}f(t)\\
%   =& -\frac{g^2(t)}{2\alpha_t} \nabla_{\bd{x}} \log p_t(\bd{x}_t|y)\\
%   =& -\frac{\frac{\dd \sigma_t^2}{\dd t} - 2 \frac{\dd \log \alpha_t}{\dd t} \sigma^2_t}{2\alpha_t} \nabla_{\bd{x}} \log p_t(\bd{x}_t|y)\\
%   =& - (\frac{1}{\alpha_t}\frac{\dd \sigma_t}{\dd t}-\frac{\sigma_t}{\alpha_t^2}\frac{\dd \alpha_t}{\dd t})\sigma_t\nabla_{\bd{x}} \log p_t(\bd{x}_t|y)\\
%   =& \frac{\dd (\sigma_t/\alpha_t)}{\dd t} \left( -\sigma_t \nabla_{\bd{x}} \log p_t(\bd{x}_t|y) \right)\\
%   =& \frac{\dd (\sigma_t/\alpha_t)}{\dd t} \bd{\epsilon}_\phi(\bd{x}_t|t, y).
%   \label{app-eq:pf-ode-simple}
% \end{aligned}
% \end{equation}
% This equation is the scaled version of Diffusion PF-ODE under the notation of Karras \etal\cite{karras2022elucidating}.
% \subsection{DDIM Sampling}
% We derive the DDIM\cite{song2020denoising} sampling algorithm in this section. According to the first order discretization of \cref{app-eq:pf-ode-simple}:
% \begin{equation}
%  \frac{\bd{x}_t}{\alpha_t} - \frac{\bd{x}_s}{\alpha_s} 
%  = (\frac{\sigma_t}{\alpha_t} - \frac{\sigma_s}{\alpha_s})
%  \bd{\epsilon}_\phi(\bd{x}_s|s, y), \label{app-eq:ddim-scale}
% \end{equation}
% the sampling algorithm of DDIM\cite{song2020denoising} can be derived as the following equation:
% \begin{equation}
%   \bd{x}_t = \alpha_t(\frac{\bd{x}_s-\sigma_s \bd{\epsilon}_\phi (x_s|y,s)}{\alpha_s}) + \sigma_t \bd{\epsilon}_\phi (\bd{x}_s|y,s). \label{app-eq:ddim}
% \end{equation}

% \subsection{Proof of Proposition 1}
% We present a detailed derivation of Proposition 1 in the main text in this section. We define
% \begin{equation}
%   \bd{x}_t = \alpha_t \xo + \sigma_t \epsf \label{app-eq:change-of-variable},
% \end{equation}
% for the reverse diffusion process and then we can apply change-of-variable on $\bd{x}_t$. Finally
% \begin{align*}
%   \frac{\dd \xo}{\dd t}
%   =& \frac{\dd \frac{\bd{x}_t - \sigma_t \epsf}{\alpha_t}}{\dd t}\\
%   =& \frac{\dd (\bd{x}_t/\alpha_t)}{\dd t} - \frac{\dd (\sigma_t/\alpha_t)}{\dd t} \epsf\\
%   =& \frac{\dd (\sigma_t/\alpha_t)}{\dd t} (\bd{\epsilon}_\phi(\bd{x}_t|t, y)-\epsf).
% \end{align*}
% We also derive first-order discretization of FSD for 2D generation from \cref{app-eq:ddim-scale}:
% \begin{equation}
%  \xo - \hat{\bd{x}}_s^o = (\frac{\sigma_t}{\alpha_t} - \frac{\sigma_s}{\alpha_s})
%  (\bd{\epsilon}_\phi(\bd{x}_s|s, y)-\epsf), \label{app-eq:fsd-1st}
% \end{equation}

% \section{Visualize the Change-of-Variable}


% \begin{figure}[pt]
%   \centering
%   \hfill
%   \begin{subfigure}{0.45\linewidth}
%     \includegraphics[width=\linewidth]{assets/same-fsd.png}\\
%     \includegraphics[width=\linewidth]{assets/same-fsd-2.png}\\
%     \includegraphics[width=\linewidth]{assets/same-fsd-3.png}
%     \caption{FSD (first-order discretization)}
%   \end{subfigure}
%   \hfill
%   \begin{subfigure}{0.45\linewidth}
%     \includegraphics[width=\linewidth]{assets/same-ddim.png}\\
%     \includegraphics[width=\linewidth]{assets/same-ddim-2.png}\\
%     \includegraphics[width=\linewidth]{assets/same-ddim-3.png}
%     \caption{DDIM\cite{song2020denoising}}
%   \end{subfigure}
%   \hfill
%   \caption{\textbf{Generation results of FSD and DDIM.} We apply FSD on 2D image generation using first-order discretization \cref{app-eq:fsd-1st} instead of Adam\cite{kingma2014adam}. In this case, we find FSD is the same as DDIM\cite{song2020denoising} except some negligible differences, which may come from the differences on handling initial conditions.
%   }
%   \label{app-fig:fsd-2d}
% \end{figure}
% Even though we show FSD can generate similar images When using the same initial noise in the main text, there are notable differences between the generated images since FSD uses Adam\cite{kingma2014adam} to update parameters while DDIM uses first-order discretization of Diffusion PF-ODE. We show generation results of FSD that use first-order discretization in \cref{app-fig:fsd-2d}.

% We also visualize the ``\textit{change-of-variable}'' trick we used in the derivation of the main theorem. We define our new variable: the \textit{clean image} $\xo$ according to the following equation:

% \begin{equation}
%   \bd{x}_t = \alpha_t \xo + \sigma_t \epsf \label{add-eq:change-of-variable}.
% \end{equation}

% Notably, there is also another similar but different concept: the \textit{one-step estimated ground-truth image} $\xc$, defined by:

% \begin{equation}
%   \bd{x}_t = \alpha_t \xc + \sigma_t \bd{\epsilon}_\phi(\bd{x}_t|y,t) \label{add-eq:predicted-clean}.
% \end{equation}

% \begin{figure}[tb]
%   \centering
%   \begin{subfigure}{0.95\linewidth}
%     \includegraphics[width=\linewidth]{assets/vis-xt.png}
%     \caption{\textit{noisy image} $\bd{x}_t$}
%   \end{subfigure}\\
%   \begin{subfigure}{0.95\linewidth}
%     \includegraphics[width=\linewidth]{assets/vis-xo.png}
%     \caption{\textit{clean image} $\xo$}
%   \end{subfigure}\\
%   \begin{subfigure}{0.95\linewidth}
%     \includegraphics[width=\linewidth]{assets/vis-xc.png}
%     \caption{\textit{one-step estimated ground-truth image} $\xc$}
%   \end{subfigure}\\
%   \caption{\textbf{Visualization of $\bd{x}_t$, $\xo$ and $\xc$ in DDIM generation process.} $\xo$ is different from $\xc$. Moreover, one can see DDIM generation process as aligning $\xo$ with $\xc$ since $\xc-\xo \propto \nabla_\theta\Lfsd$ 
%   }
%   \label{app-fig:vars}
% \end{figure}
% \begin{figure}[htp]
%   \centering
%   \begin{subfigure}{0.95\linewidth}
%     \includegraphics[width=\linewidth]{assets/vis-xt-fsd.png}
%     \caption{\textit{noisy image} $\bd{x}_t$}
%   \end{subfigure}\\
%   \begin{subfigure}{0.95\linewidth}
%     \includegraphics[width=\linewidth]{assets/vis-xo-fsd.png}
%     \caption{\textit{clean image} $\xo$}
%   \end{subfigure}\\
%   \begin{subfigure}{0.95\linewidth}
%     \includegraphics[width=\linewidth]{assets/vis-xc-fsd.png}
%     \caption{\textit{one-step estimated ground-truth image} $\xc$}
%   \end{subfigure}\\
%   \caption{\textbf{Visualization of $\bd{x}_t$, $\xo$ and $\xc$ in FSD generation process.} Compared to DDIM, FSD uses Adam\cite{kingma2014adam} to update parameters. As a result, FSD needs more iterations to converge (See \cref{app-tab:impl-2d}).
%   }
%   \label{app-fig:vars-fsd}
% \end{figure}
% \begin{figure}[htp]
%   \centering
%   \begin{subfigure}{0.95\linewidth}
%     \includegraphics[width=\linewidth]{assets/vis-xt-sds.png}
%     \caption{\textit{noisy image} $\bd{x}_t$}
%   \end{subfigure}\\
%   \begin{subfigure}{0.95\linewidth}
%     \includegraphics[width=\linewidth]{assets/vis-xo-sds.png}
%     \caption{\textit{clean image} $\xo$}
%   \end{subfigure}\\
%   \begin{subfigure}{0.95\linewidth}
%     \includegraphics[width=\linewidth]{assets/vis-xc-sds.png}
%     \caption{\textit{one-step estimated ground-truth image} $\xc$}
%   \end{subfigure}\\
%   \caption{\textbf{Visualization of $\bd{x}_t$, $\xo$ and $\xc$ in SDS generation process.} Compared to FSD, SDS adds random noise instead of fixed noise. As a result, the estimated GT images vary a lot and SDS needs a larger learning rate to converge (See \cref{app-tab:impl-2d}). 
%   }
%   \label{app-fig:vars-sds}
% \end{figure}
% We visualize the trajectory of $\bd{x}_t$, $\xo$ and $\xc$ in the same DDIM generation process in \cref{app-fig:vars}. As $\xc-\xo = \frac{\sigma_t}{\alpha_t} (\epsf-\bd{\epsilon}_\phi(\bd{x}_t|y,t)) \propto \nabla_\theta\Lfsd$ implies, we can see DDIM as a process that tries to align \textit{clean image} with the \textit{one-step estimated ground-truth image} generated by the Diffusion Model. We also visualize $\bd{x}_t$, $\xo$ and $\xc$ of FSD and SDS in \cref{app-fig:vars-fsd} and \cref{app-fig:vars-sds}, respecitively.


% \section{Algorithm for Flow Score Distillation}
% We provide a summarized algorithm for Flow Score Distillation in \cref{app-alg:fsd}.

% \begin{algorithm}[H]
% \begin{algorithmic}[1]
% \STATE \textbf{Input:} Text-to-image Diffusion Model $\bd{\epsilon}_\phi$ and prompt $y$. Learning rate $\eta$ for parameters of the 3D representation. A monotonically decreasing function $t(\tau)$. Blending factor $\beta$.
% \STATE Compute $\bd{\epsilon}_b \sim \Normal$ and $\bd{\epsilon}_p \sim \Normal$.
% \FOR{$\tau \in [0, \tau_{\text{end}}]$}
%     \STATE Randomly sample camera parameter $\bd{c}$.
%     \STATE Render image $\gc$ and opacity mask $\bd{M}$ from 3D representation $\theta$.
%     \STATE Randomly sample $\bd{\epsilon}\sim\Normal$.
%     \STATE $\ec \leftarrow \sqrt{\beta} \cdot \left( (1-\bd{M}) \odot \bd{\epsilon}_b + \bd{M} \odot \window(\bd{\epsilon}_p) \right) + \sqrt{1-\beta} \cdot \bd{\epsilon}$.
%     \STATE $\theta \leftarrow \theta - \eta \cdot (\bd{\epsilon}_\phi(\bd{x}_t|y,t) - \ec)\frac{\partial \gc}{\partial \theta}$
% \ENDFOR
% \end{algorithmic}

% \caption{Flow Score Distillation}
% \label{app-alg:fsd}
% \end{algorithm}

% \section{Practical Designing Rules for $\bd{\epsilon}(\bd{c})$}
% \subsection{Practical Designing Rules}
% We do not specify the form of $\ec$ in the general form of FSD in the main text. However, it is intuitive to align $\ec$ in 3D space like the noise priors used in Video Diffusion Models\cite{chang2024how, ge2023preserve, qiu2023freenoise}. We have tried several designs of $\ec$ and summarized several design rules for designing $\ec$ as well as the related potential problems if violating the design rules for $\ec$:

% \begin{itemize}
%     \item The noise associated with each camera view conditioning on camera view should be an uncorrelated Gaussian noise. \ie $\ec|\bd{c}\sim\Normal$. If not so, the input image may be out-of-distribution for the pretrained text-to-image Diffusion Models.
%     \item The noise associated with different camera views should be aligned in 3D space. Otherwise, FSD may degrade to the original SDS. This is consistent with the observation of recent work\cite{ge2023preserve} on Video Generation, which showed that the noise maps corresponding to different video frames are highly correlated.
%     \item The noise should not be only aligned in specific points in the 3D space. This may lead to broken geometry since the convergence speed in 3D space is not uniform (see analysis on failure of constant noise function in the main text). 
% \end{itemize}

% \subsection{World-map Noise Function}
% We will take a deeper analysis of the property of the world map noise function in the main text. We will discuss how our proposed design rules are followed.

% As noted in the main text, the local texture of the added noise is highly correlated with the generated images. In 3D spaces, it is natural to identify points, that correspond to similar points on the noise maps when projected onto the image planes of different camera views $\bd{c}$, as the points of high convergence speed. Let us denote those points as $\bd{p}_+$. For simplicity, we study the $\bd{p}_+$ that corresponds to the center points in image space.

% For object-centric generation, a common camera view sampling strategy is to sample camera positions at $(r_{\text{cam}},\theta_{\text{cam}}, \phi_{\text{cam}})$ under spherical coordinate and force the camera to look at the center point. When we apply a constant noise function as $\ec$, the center point in 3D space is a $\bd{p}_+$ point. As a result, FSD trends to generate geometry with holes. When applying world-map noise function proposed in main text, $\bd{p}_+$ is located at $(r_+,\theta_{\text{cam}}, \phi_{\text{cam}})$. One can compute that 
% \begin{equation}
%     r^{\theta_{\text{cam}}}_+\approx\frac{2 \tan \frac{\text{FOV}}{2}}{2 \tan \frac{\text{FOV}}{2} + \Theta}\cdot r_{\text{cam}} \label{app-eq:rp-theta}
% \end{equation}
% if consider nearby views with slightly different $\theta_{\text{cam}}$ and 
% \begin{equation}
%     r^{\phi_{\text{cam}}}_+\approx\frac{2 \tan \frac{\text{FOV}}{2}}{2 \tan \frac{\text{FOV}}{2} + \Theta \cdot \sin \theta_{\text{cam}}}\cdot r_{\text{cam}}  \label{app-eq:rp-phi}
% \end{equation}
% if consider views with slightly different $\phi_{\text{cam}}$. In this way, 
% we align nearby views coarsely. Moreover, for different camera parameters, $r_+$ is different, avoiding nonuniform convergence speed in 3D space.

% \bibliographystyle{splncs04}
% \bibliography{main}

% \end{document}
